# Supplementary material for: Non-rigid 3D motion estimation at high temporal resolution from prospectively undersampled k-space data using low-rank MR-MOTUS
Source: arXiv:2007.00488 source file (2020-07-01)
Supplement: Supplementary file 2 [file SupportingInformation.pdf]

# Supplementary Information

## 1 Extension of MR-MOTUS to multi-coil acquisitions

In ( ? ), the model in ?? was derived by substituting

$$q_t(\mathbf{x}) = q_0(\mathbf{U}_t(\mathbf{x})) \det \nabla(\mathbf{U}_t(\mathbf{x})) \quad [\text{S1}]$$

in the conventional MRI signal equation

$$s_t(\mathbf{k}) = \int_{\Omega} q_t(\mathbf{x}) e^{-i2\pi\mathbf{k}\cdot\mathbf{x}} d\mathbf{x}, \quad [\text{S2}]$$

followed by a change-of-variables. Since  $\mathbf{q}_t(\mathbf{x})$  is defined as the transverse magnetization at time  $t$ , ?? is based on the assumption that the coil sensitivities are smooth throughout the whole FOV.

In a multi-coil acquisition, k-space data  $s_t^j(\mathbf{k})$  from coil  $j$  with coil sensitivity  $S^j(\mathbf{x}) \in \mathbb{C}$  can be modelled as

$$s_t^j(\mathbf{k}) = \int_{\Omega} S^j(\mathbf{x}) q_t(\mathbf{x}) e^{-i2\pi\mathbf{k}\cdot\mathbf{x}} d\mathbf{x}. \quad [\text{S3}]$$

Hence, the signal model [??] cannot be employed for multi-coil acquisitions, and consequently the model and reconstruction techniques introduced in ( ? ) cannot be employed directly.

To extend the framework to handle multi-coil data, we design a coil compression strategy that reduces all multi-channel data to a single channel with approximately homogeneous sensitivity. This allows to use the same reconstruction strategy for multi-coil data as for single-channel data. Since the targeted application of this work is on MR-LINAC systems that operate on 1.5T, coil sensitivities can be assumed smooth and slowly varying, such that global coil weightings could be sufficient to achieve homogeneous sensitivity. Such global coil weightings  $c^j \in \mathbb{C}$  should satisfy

$$\sum_{j=1}^{N_c} c^j S^j(\mathbf{x}) \approx 1, \quad \forall \mathbf{x} \in \mathbb{R}^d, \quad [\text{S4}]$$

where  $N_c$  denotes the number of coils. We also desire coefficients that yield high SNR after compression. Combining both requirements, the compression coefficients can be obtained by solving the following minimization problem

$$\min_{\mathbf{c}} \|\mathbf{S}\mathbf{c} - \mathbf{1}\|_2^2 + \lambda_{cc} \|\mathbf{U}\mathbf{c}\|_2^2. \quad [\text{S5}]$$

Here  $\mathbf{S} \in \mathbb{C}^{N \times N_c}$  denotes the matrix of coil sensitivities,  $\mathbf{1} \in \mathbb{C}^{N \times 1}$  denotes a vector with all entries equal to one, and  $\mathbf{U}$  denotes Cholesky factor of the noise covariance matrix  $\mathbf{\Sigma}$  such that  $\mathbf{\Sigma} = \mathbf{U}^H \mathbf{U}$ . The minimization problem in ?? has a unique solution given by

$$\mathbf{c} = [\mathbf{S}^H \mathbf{S} + \lambda_{cc} \mathbf{\Sigma}]^{-1} \mathbf{S}^H \mathbf{1}, \quad [\text{S6}]$$

where the superscript  $H$  denotes the conjugate transpose.

Applying the compression coefficients in ?? to both sides of ?? yields:

$$\tilde{\mathbf{s}}_t = \mathbf{F}(\mathbf{D}_t | \tilde{\mathbf{q}}_0). \quad [\text{S7}]$$

Here  $\tilde{\mathbf{s}}_t := \sum_j c^j \mathbf{s}_t^j$  and  $\tilde{\mathbf{q}}_0 := \sum_j c^j S^j(\mathbf{x}) \mathbf{q}_0(\mathbf{x}) \approx \mathbf{q}_0(\mathbf{x})$  denote the coil-compressed k-space data and reference image, respectively, and can be pre-computed before the motion-field reconstruction. Note that this includes the same operator as in ??, such that the same reconstruction strategy as for single-channel data can now be employed to reconstruct motion-fields from multi-coil acquisitions. This thus allows for similar reconstruction times with multi-coil data, but comes at the cost of SNR loss. For all experiments considered in this work we have set the compression parameter  $\lambda_{CC} = 5 \cdot 10^5$ ; this yielded an empirically good trade-off between SNR loss and homogeneous sensitivities.

As mentioned above, the proposed compression is not optimal in terms of SNR ( ? ? ). To this extent, ?? analyzes the loss in SNR between a Roemer coil combination ( ? ) and the proposed coil compression on the 2D respiratory data. This shows an SNR loss factor between 1.5 and 2.5 in most of the body, which increases towards the boundary of the body. k-Space-based parallel imaging methods such as GRAPPA could possibly be used to improve the SNR after the compression.

## 2 Reference image reconstruction from free-breathing, multi-coil acquisitions

MR-MOTUS requires a motion-free reference image with slowly varying coil sensitivity. To be consistent with the forward model in ??, the reference image  $\tilde{\mathbf{q}}_0$  should be reconstructed from the data  $\tilde{\mathbf{s}}_t$  after coil compression. This data was, however, acquired during free-breathing which makes

the reconstruction of a motion-free image not trivial. The extreme positions in the respiratory motion (i.e. end-inhale, end-exhale) can be assumed relatively constant over different breathing cycles. To extract motion-free k-space data from the free-breathing data, we retrospectively selected only the readouts acquired at end-inhale; this yielded consistently better results than end-exhale. To enable this selection, we performed phase-binning on every readout based on the magnitude of the signal at  $\mathbf{k} = \mathbf{0}$  (denoted as  $k_0$ -values). A low-pass filter was applied to the time-series of  $k_0$ -values prior to the binning, based on the expected breathing frequency. Next, phase-binning was performed with 10 phases per breathing cycle. Finally, the reference image was reconstructed from the end-inhale bin, using a density-compensated preconditioned conjugate-gradient reconstruction.

### 3 Heuristic search for reconstruction parameter settings

We have heuristically determined the reconstruction parameter settings based on the quality of the respiratory-resolved MR-MOTUS reconstructions described in ???. The number of dynamics was set equal to the number of bins, i.e. 20, and as a quality metric we have taken the maximum REN between the reconstructions over all 20 dynamics. This allowed to select the parameters with the best worst-case performance over all respiratory phases. The reconstruction parameters included the resolution of the reference image, the binning-phase of the reference image, the spline order for the motion-field basis and the number of motion model components  $R$ . The optimal reconstruction parameters were determined as follows. First, the spline order was fixed to 9 (i.e. 9 spline functions over the whole FOV, in every direction), in order to have at least the 4 points required to correctly define a single third order B-spline on every resolution level. A grid search was then performed for the reference image resolution, binning-phase and the number of motion model components, with as metric the maximum REN over all dynamics. Next, the optimal parameters resulting from the grid search were selected, the spline order was increased to the maximum (i.e. 1 spline function per 4 grid-points), and a second grid search was performed for only the regularization parameter  $\lambda_R$ . To vary the spatial resolution of the reference image we have retrospectively varied the  $k_{\max}$  of the data, resulting in varying matrix sizes and, consequently, reconstruction times. To vary the respiratory-phase, the binning as described in ??? is performed to select only the required phase.

??? visualizes the quantitative results of the parameter search. ???A shows the REN of the worst-

case dynamic, minimized over the number of motion model components ( $R = 1 - 6$ ), versus the reference image resolution. No regularization was applied yet. The best worst-case performance was obtained for a reference image resolution binned in end-inhale with a spatial resolution of 6.7 mm isotropic, and motion model with  $R = 3$ . This reference resolution was subsequently fixed, the motion resolution was set to the maximum of 1 spline function per 4 grid-points (i.e. spline order 16), and the optimal value for the regularization parameter was determined with a grid-search. This resulted in an optimum value of  $\lambda_R = 15$ . ?? qualitatively compares the MR-MOTUS reconstructions with respiratory-resolved image reconstructions for different reference image binning-phases and reference image resolution. Although the visual differences between the reconstructions are minimal, it can be observed from ??B that the reconstruction times are about a factor 3 lower for a reference image resolution of 6.7 mm, than for a resolution of 3.4 mm.

?? shows the comparison for the average kidney motion. The phase of the reconstructions are most similar for the feet-head (FH) and anterior-posterior (AP), and these axes also correspond to the largest motion magnitude. The left-right (LR) axis shows very different patterns, but it should be noted that the motion is two orders of magnitude lower than the FH and AP axes. The magnitude of the motion is similar for both reconstructions, but by construction, the respiratory-resolved reconstruction shows a constant amplitude over time since it only reconstructs an average breathing cycle. The time-resolved reconstruction shows changing motion amplitudes over time. The phase difference between the two reconstructions may be explained by imperfect respiratory-sorting.

## 4 Embarrassingly parallel implementation of forward operator and adjoint

The forward model in [??], and corresponding derivatives (see Supplementary Information in ( ? )) required for the motion-field reconstruction problem [??] are computed using the NUFFT-operator from ( ? ). We observe that the evaluation of the data-fidelity term  $E[\cdot]$  in the objective function [??] includes a sum over  $M$  independent terms. We found that a so-called ‘embarrassingly parallel’ evaluation of the data-fidelity term can result in a reduced computation time. This requires a single-thread compilation of the NUFFT, and a parallelization over the  $M$  independent terms in

the summation. The parallization was realized in MATLAB with a ‘parfor-loop’ over the dynamics. For 3D this resulted in a significant improvement in computation times, while for 2D the speed-up due to parallelization was smaller than the thread initialization overhead. Hence, for 2D we consider the non-parallelized evaluation and for 3D we consider the parallelized evaluation.

## Supplementary Figures

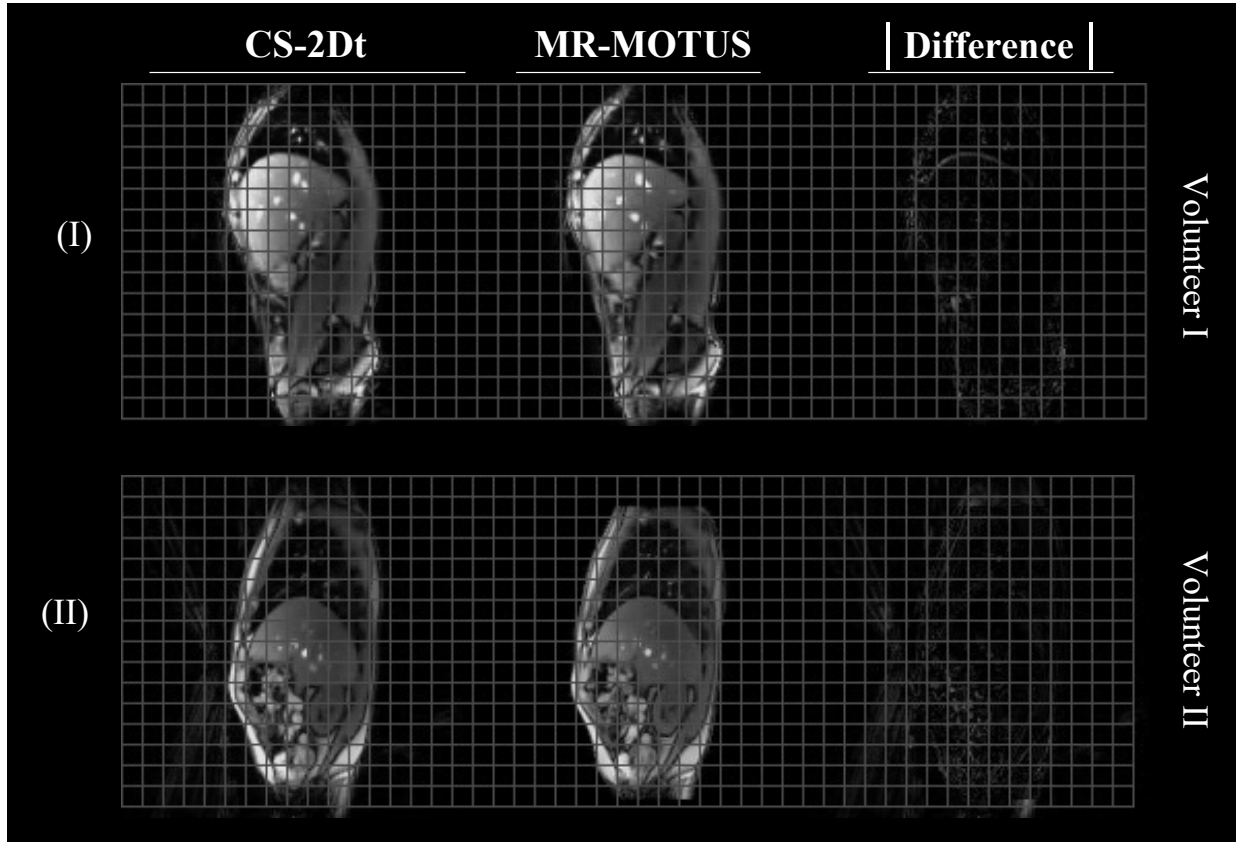

**Supporting Information Video S1:** *This is an animated figure and should be viewed at <https://surfdrive.surf.nl/files/index.php/s/XcXY3cHETnmXtY0>. 2D-t compressed sensing reconstruction (left), MR-MOTUS warped reference images (middle), and pixel-wise absolute differences between the two reconstructions (right), as mentioned in ?? and ??. The top row shows reconstructions for volunteer 1, and the bottom row for volunteer 2.*

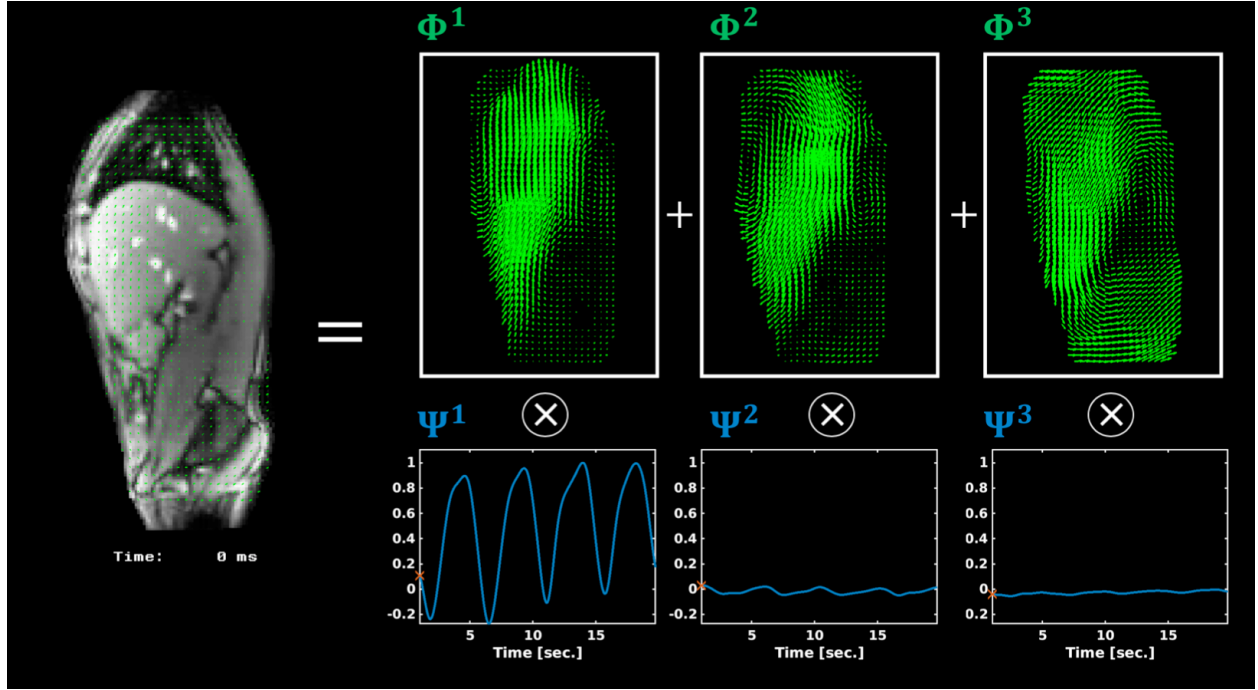

**Supporting Information Video S2:** *This is an animated figure and should be viewed at <https://surfdrive.surf.nl/files/index.php/s/XcXY3cHETnmXtY0>. MR-MOTUS warped reference images overlayed with reconstructed dynamic motion-fields from 2D time-resolved data, as mentioned in ?? and ??. The image shows a decomposition in the reconstructed components  $\Phi^i$  (spatial) and  $\Psi$  (temporal) for volunteer 1. For visualization purposes the components were scaled such that  $\|\Phi^i\| = 1$ .*

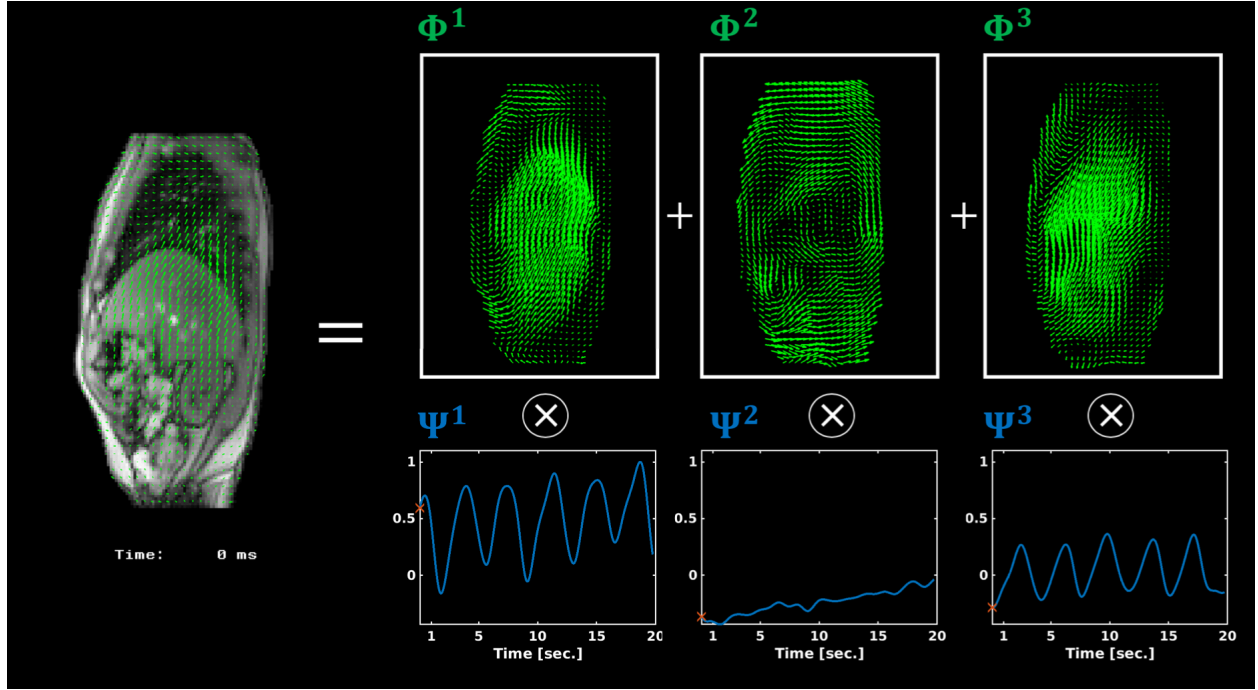

**Supporting Information Video S3:** *This is an animated figure and should be viewed at <https://surfdrive.surf.nl/files/index.php/s/XcXY3cHETnmXtY0>. MR-MOTUS warped reference images overlaid with reconstructed dynamic motion-fields from 2D time-resolved data, as mentioned in ?? and ??. The image shows a decomposition in the reconstructed components  $\Phi^i$  (spatial) and  $\Psi$  (temporal) for volunteer 2. For visualization purposes the components were scaled such that  $\|\Phi^i\| = 1$ .*

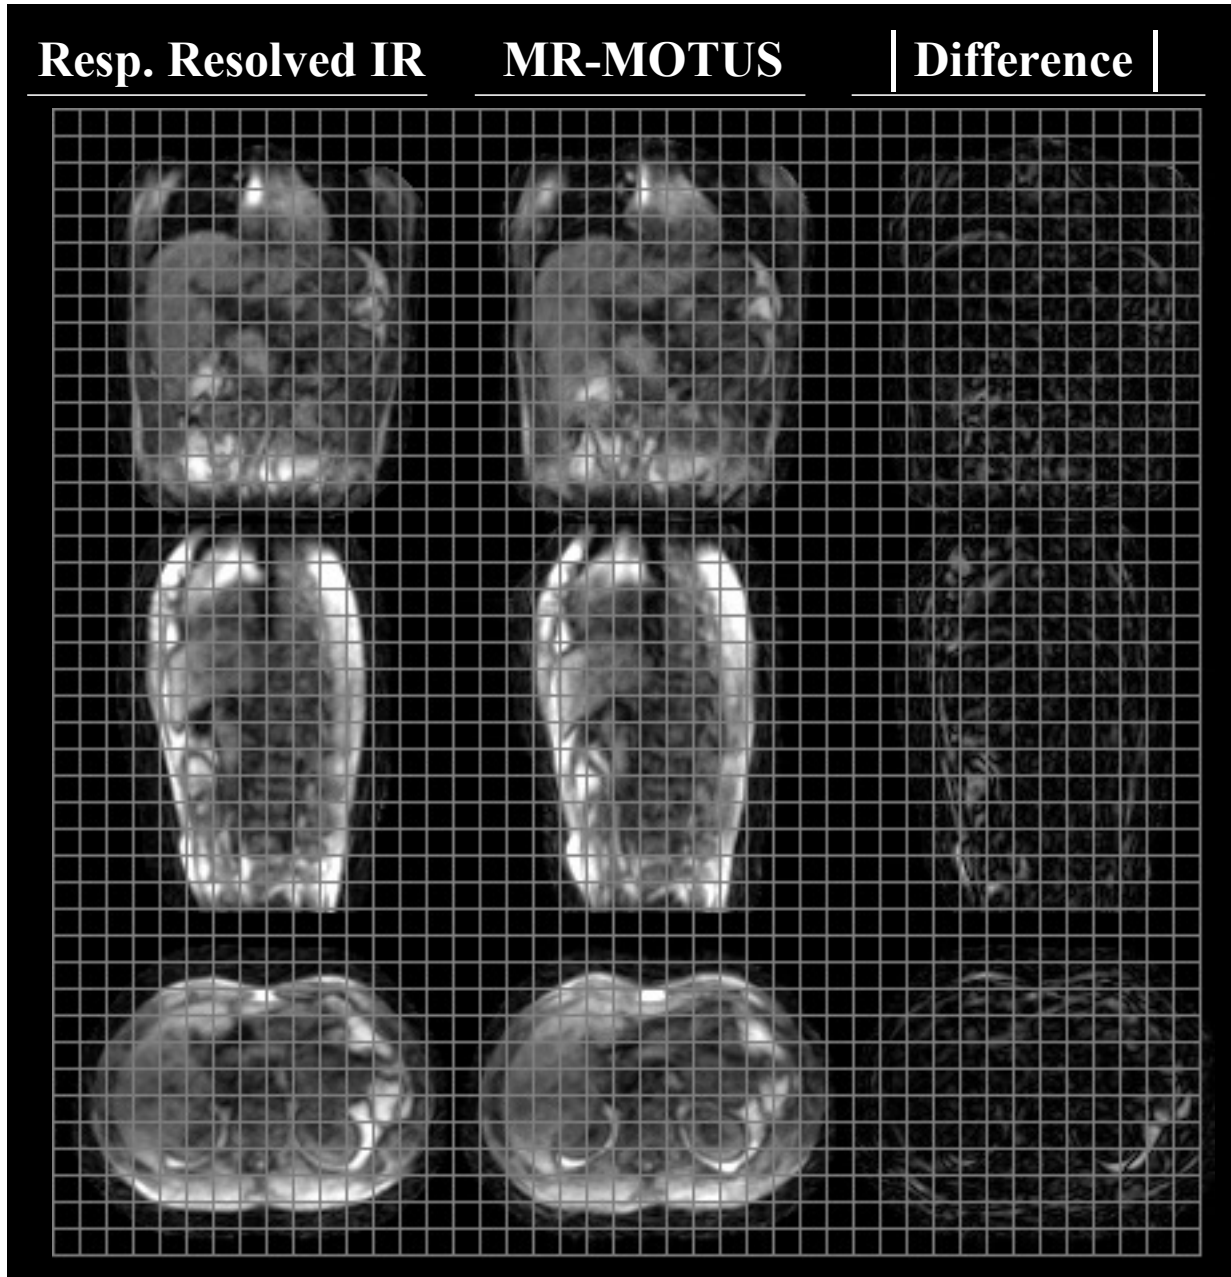

**Supporting Information Video S4:** *This is an animated figure and should be viewed at <https://surfdrive.surf.nl/files/index.php/s/XcXY3cHETnmXtY0>.* Respiratory-resolved image reconstruction (Resp. resolved IR, left), MR-MOTUS warped reference images (middle), and pixel-wise absolute differences between the two reconstructions (right), as mentioned in ?? and ??. The visualization shows data from volunteer 1.

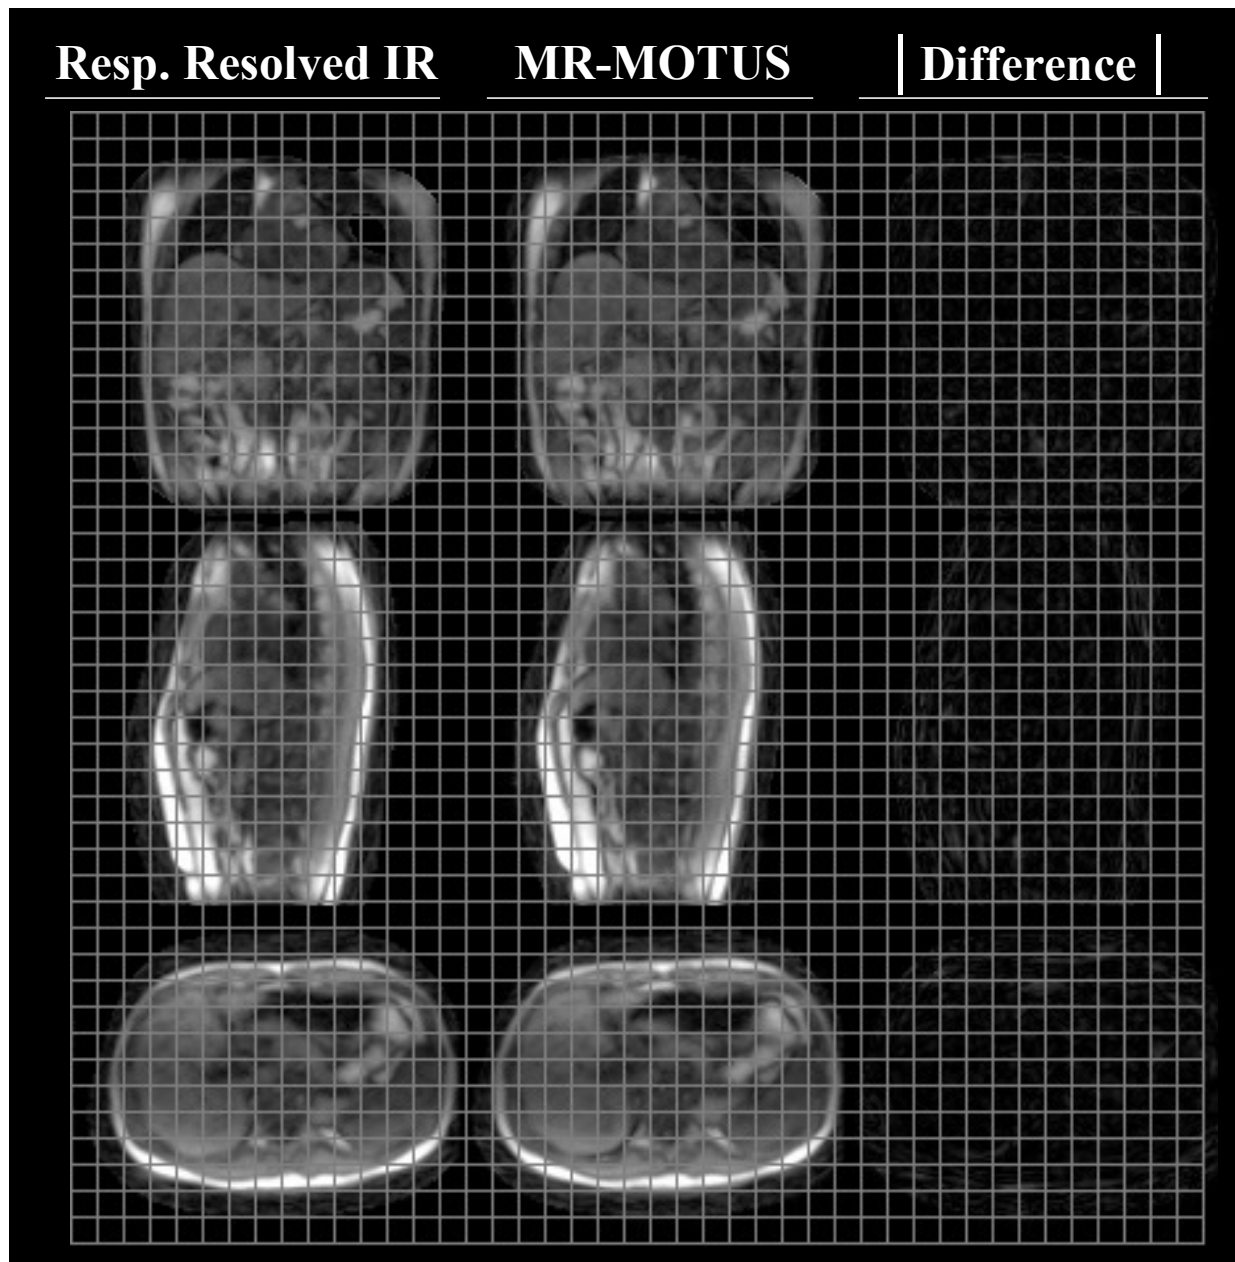

**Supporting Information Video S5:** *This is an animated figure and should be viewed at <https://surfdrive.surf.nl/files/index.php/s/XcXY3cHETnmXtY0>. Respiratory-resolved image reconstruction (Resp. resolved IR, left), MR-MOTUS warped reference images (middle), and pixel-wise absolute differences between the two reconstructions (right), as mentioned in ?? and ??. The visualization shows data from volunteer 2.*

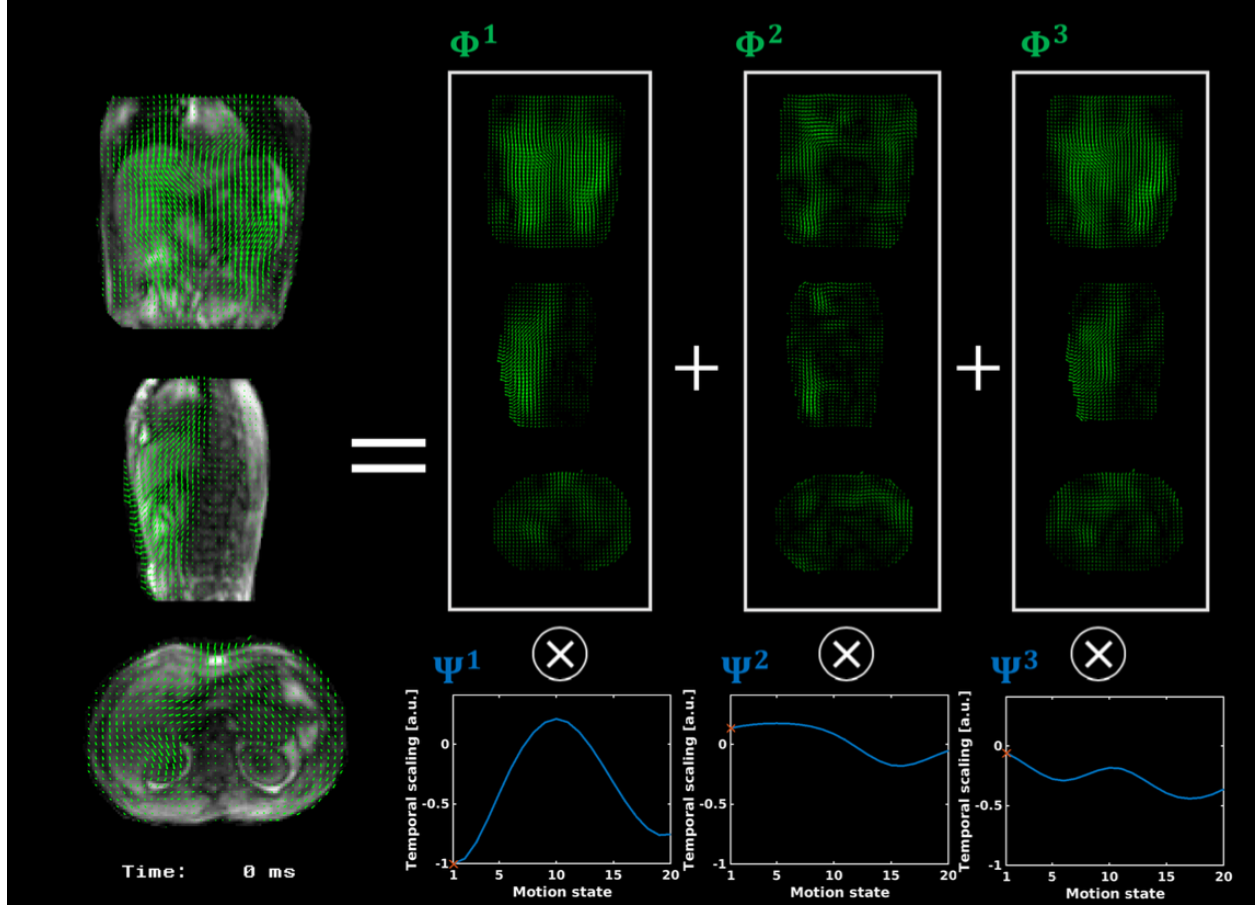

**Supporting Information Video S6:** *This is an animated figure and should be viewed at <https://surfdive.surf.nl/files/index.php/s/XcXY3cHETnmXtY0>. MR-MOTUS warped reference images overlaid with reconstructed dynamic motion-fields from respiratory-sorted data, as mentioned in ?? and ??. The image shows a decomposition in the reconstructed components  $\Phi^i$  (spatial) and  $\Psi$  (temporal) for volunteer 1. For visualization purposes the components were scaled such that  $\|\Phi^i\| = 1$ .*

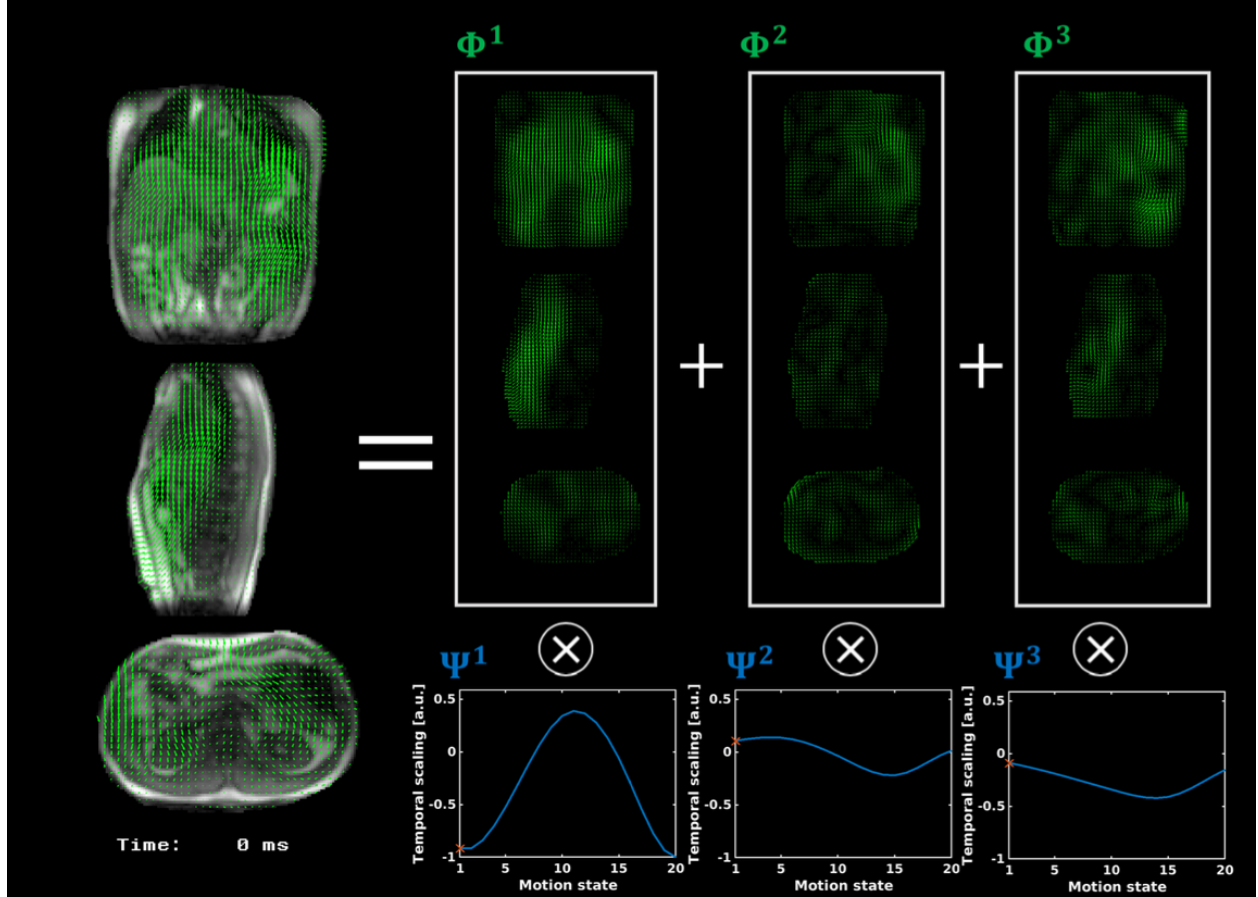

**Supporting Information Video S7:** *This is an animated figure and should be viewed at <https://surfdrive.surf.nl/files/index.php/s/XcXY3cHETnmXty0>. MR-MOTUS warped reference images overlaid with reconstructed dynamic motion-fields from respiratory-sorted data, as mentioned in ?? and ??. The image shows a decomposition in the reconstructed components  $\Phi^i$  (spatial) and  $\Psi$  (temporal) for volunteer 2. For visualization purposes the components were scaled such that  $\|\Phi^i\| = 1$ .*

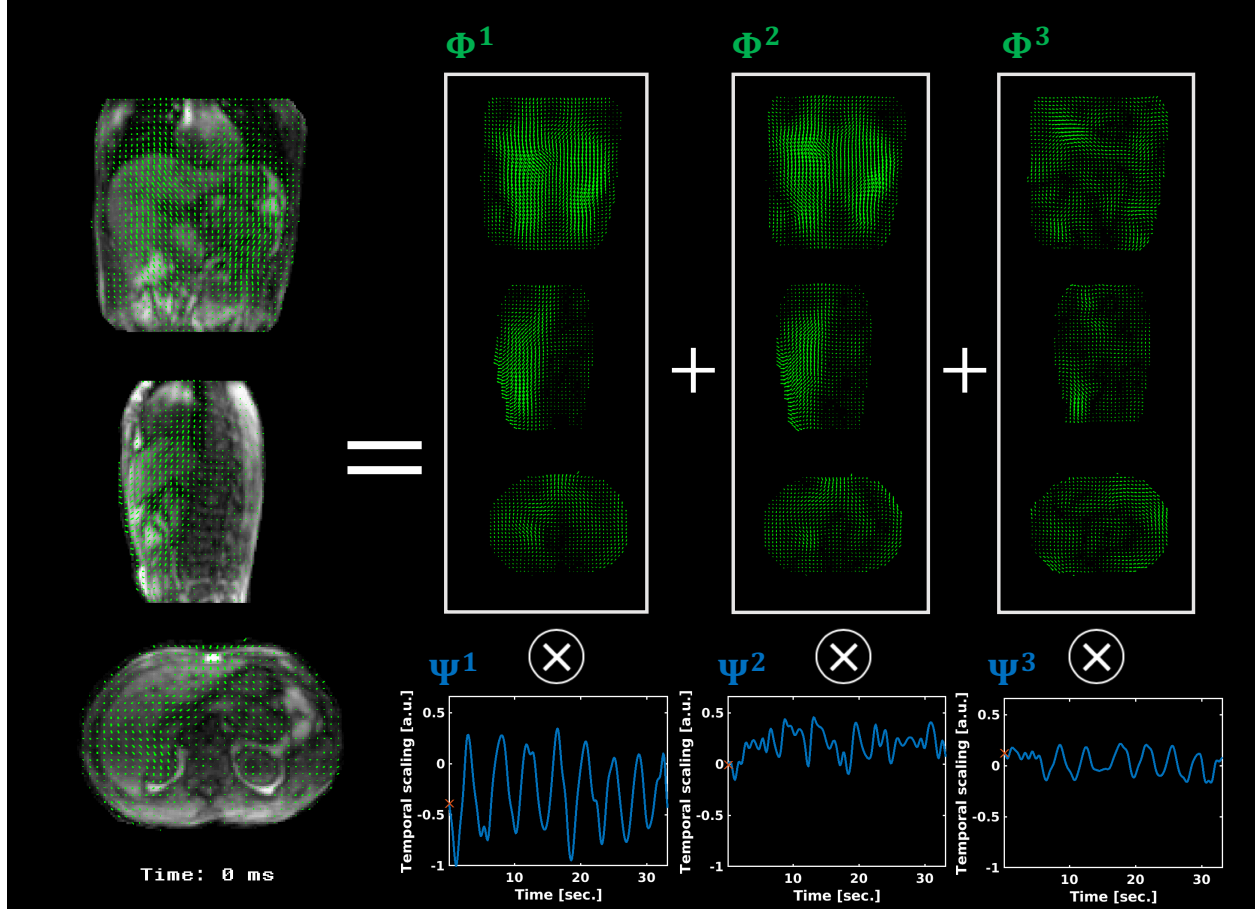

**Supporting Information Video S8:** *This is an animated figure and should be viewed at <https://surfdrive.surf.nl/files/index.php/s/XcXY3cHETnmXtY0>. MR-MOTUS warped reference images overlaid with reconstructed dynamic motion-fields from respiratory-sorted data, as mentioned in ?? and ??. The image shows a decomposition in the reconstructed components  $\Phi^i$  (spatial) and  $\Psi$  (temporal) for volunteer 1. For visualization purposes the components were scaled such that  $\|\Phi^i\| = 1$ .*

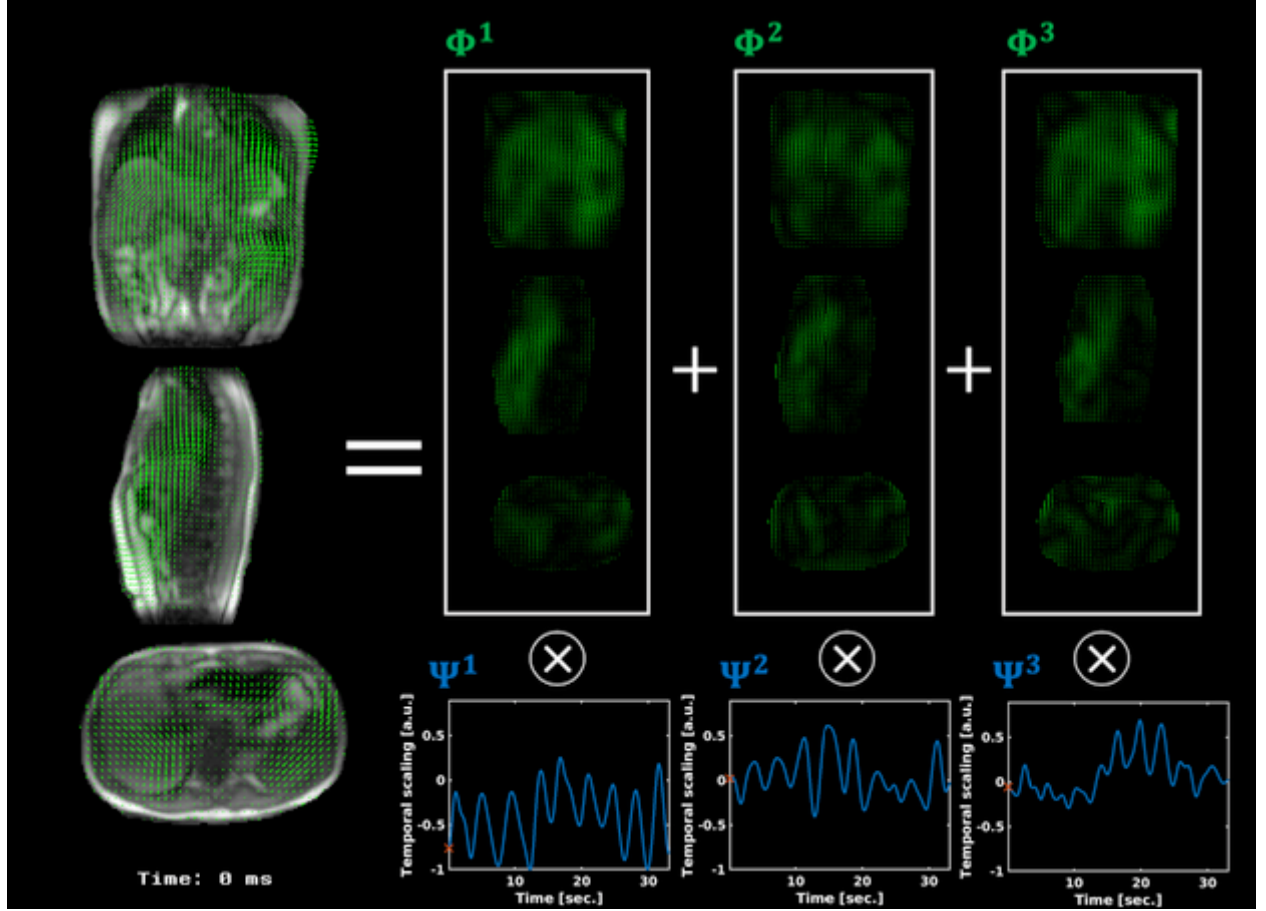

**Supporting Information Video S9:** *This is an animated figure and should be viewed at <https://surfdrive.surf.nl/files/index.php/s/XcXY3cHETnmXtY0>. MR-MOTUS warped reference images overlaid with reconstructed dynamic motion-fields from respiratory-sorted data, as mentioned in ?? and ??. The image shows a decomposition in the reconstructed components  $\Phi^i$  (spatial) and  $\Psi$  (temporal) for volunteer 2. For visualization purposes the components were scaled such that  $\|\Phi^i\| = 1$ .*

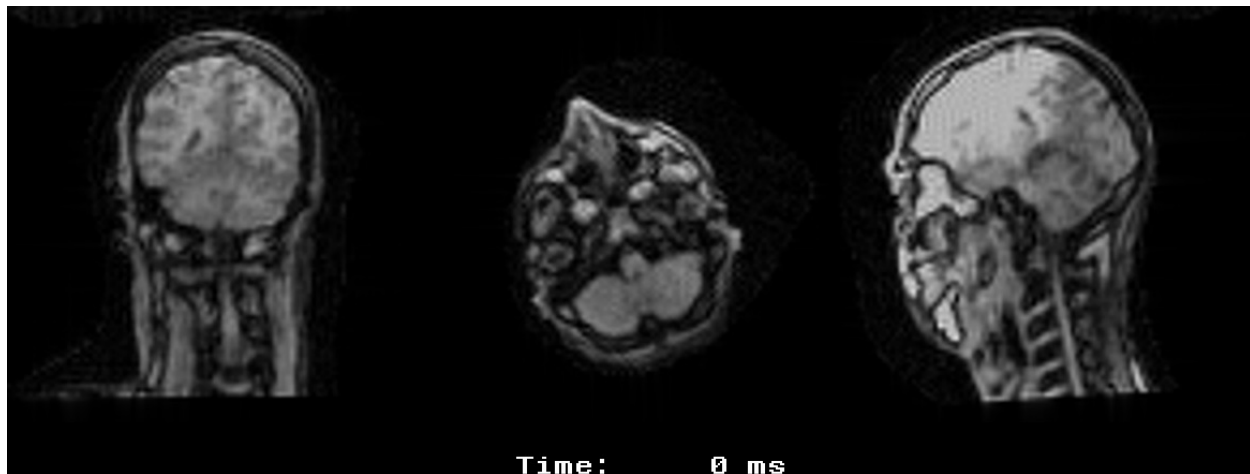

**Supporting Information Video S10:** *This is an animated figure and should be viewed at <https://surfdrive.surf.nl/files/index.php/s/XcXY3cHETnmXtY0>. MR-MOTUS warped reference images resulting from the 3D head-and-neck motion reconstructions for volunteer 1, as mentioned in ?? and ??.*

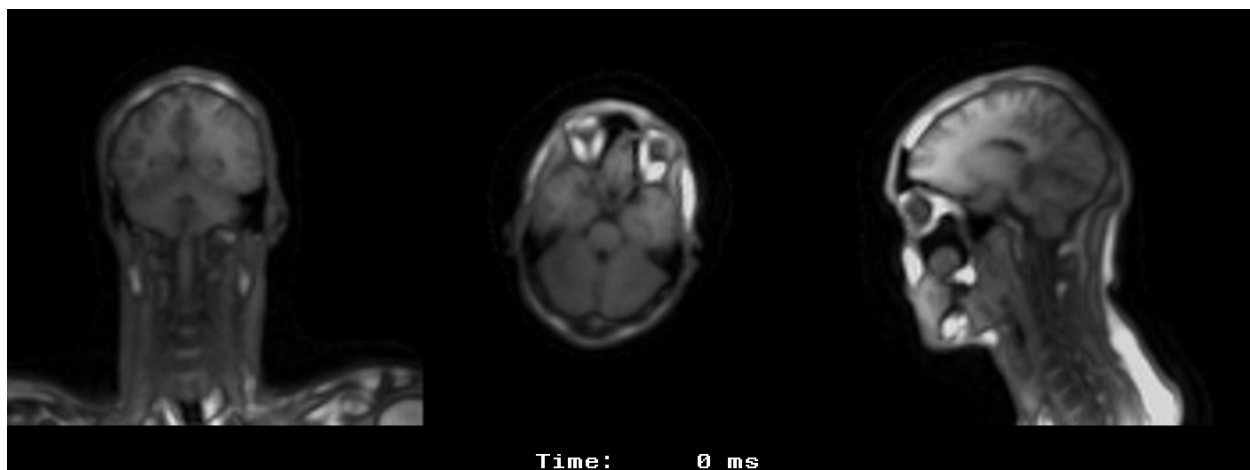

**Supporting Information Video S11:** *This is an animated figure and should be viewed at <https://surfdrive.surf.nl/files/index.php/s/XcXY3cHETnmXtY0>. MR-MOTUS warped reference images resulting from the 3D head-and-neck motion reconstructions for volunteer 2, as mentioned in ?? and ??.*

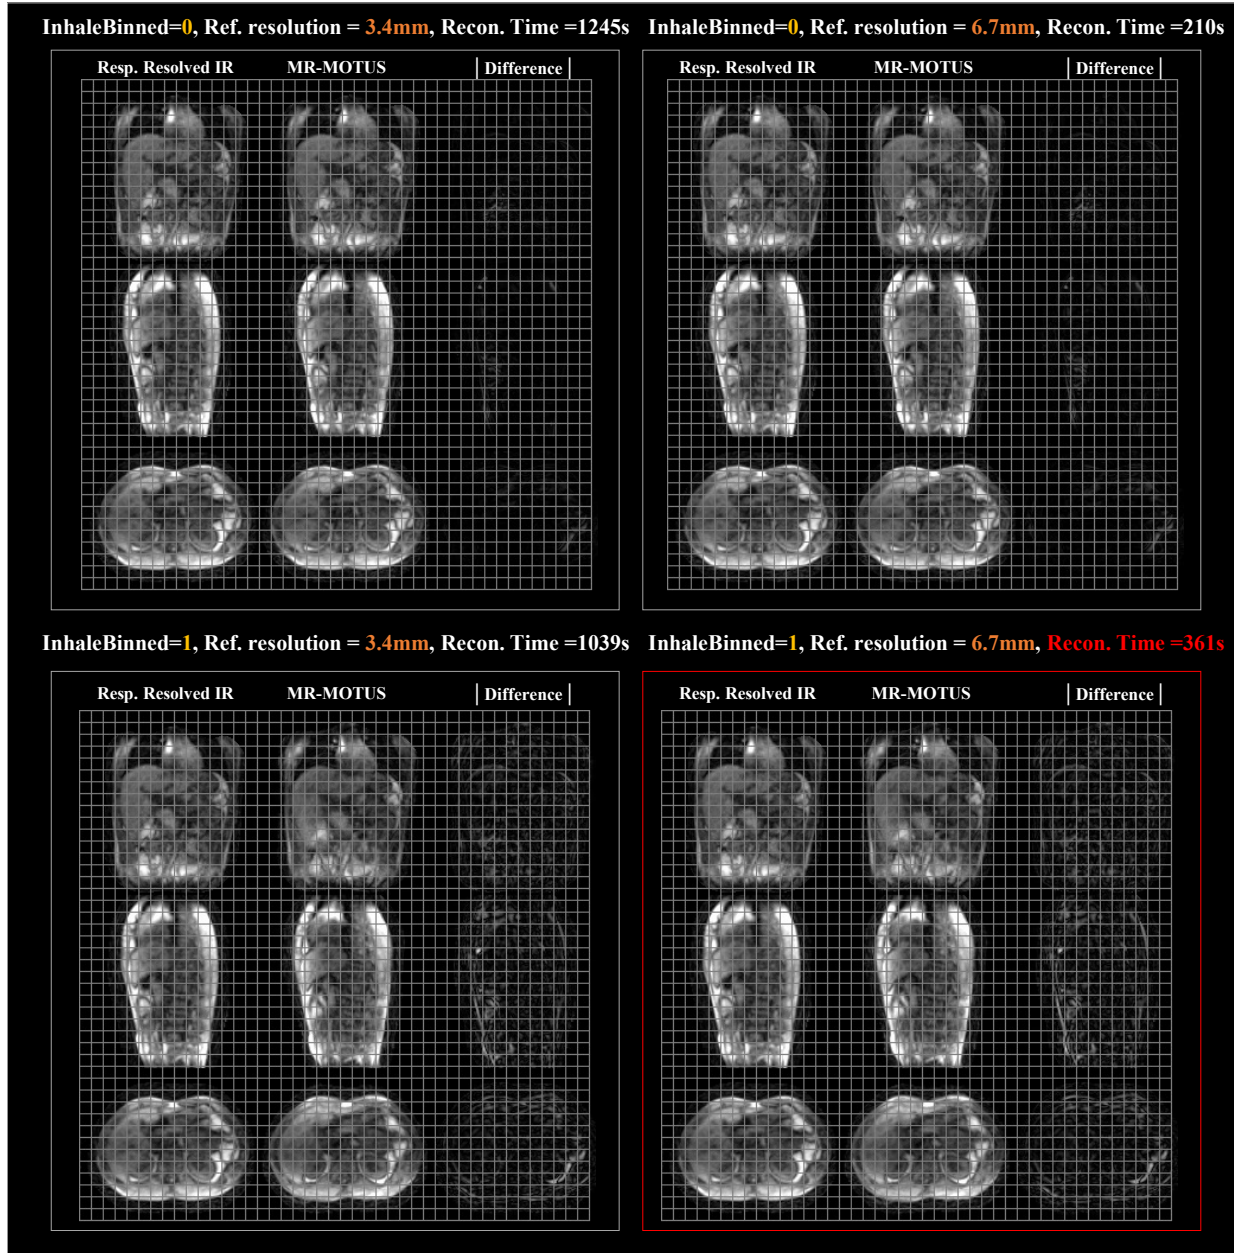

**Supporting Information Video S12:** *This is an animated figure and should be viewed at <https://surfdrive.surf.nl/files/index.php/s/XcXY3cHETnmXtY0>.* Respiratory-resolved image reconstruction (Resp. resolved IR, left), MR-MOTUS warped reference images (middle), and pixel-wise absolute differences between the two reconstructions (right), as mentioned in ?? and ??. The four blocks show reconstructions with different reconstruction parameter settings. ‘InhaleBinned’ denotes whether the reference image is binned in inhale (1) or exhale (0). ‘Ref. resolution’ denotes the resolution of the reference image in millimeters. All motion-fields were reconstructed without regularization and with 9 cubic spline functions in every direction.

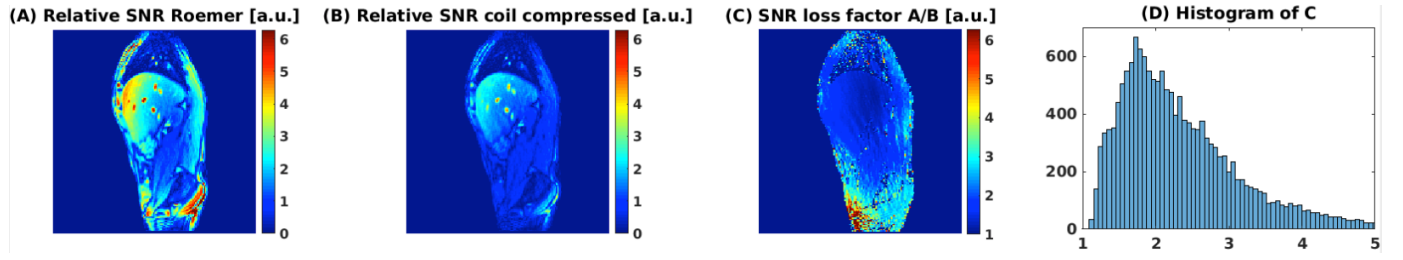

**Supporting Information Figure S13:** (A) Roemer reconstruction (? ). (B) The coil compression with  $\lambda_{CC} = 5 \cdot 10^5$ , as discussed in ?? . (C) SNR loss factor between (A) and (B). (D) The histogram of the SNR loss factor in (C). The SNR loss factor is between 1.5 and 2.5 in most of the body and increases towards the boundary of the body.

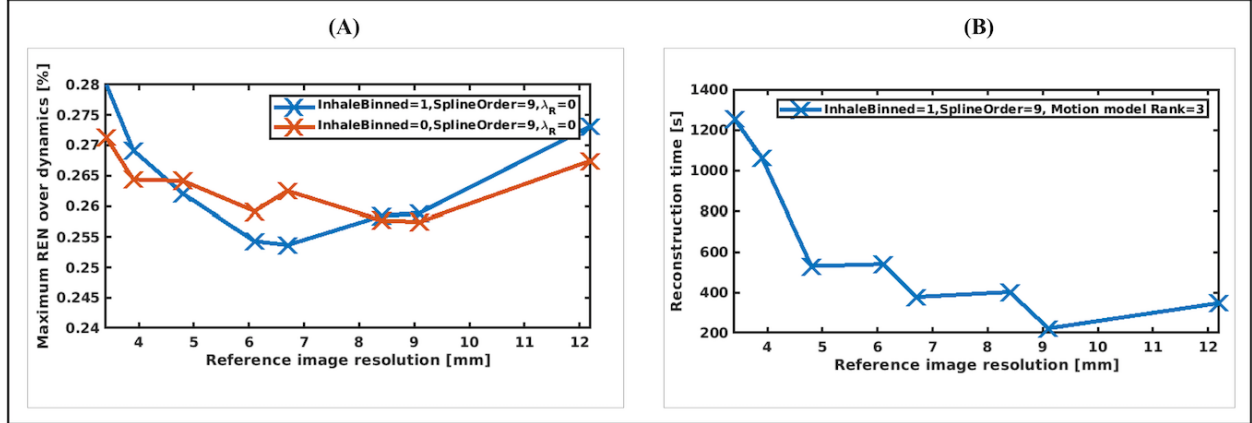

**Supporting Information Figure S14:** Results of the parameter search as mentioned in ?? and ??. (A) The effect of the reference image resolution and reference image respiratory binning-phase on the reconstruction quality. (B) The effect of the reference image resolution on the reconstruction time. In the figure, ‘InhaleBinned’ refers to the binning phase for the reference image (InhaleBinned=1 for inhale, InhaleBinned=0 for exhale), ‘Resolution’ denotes the spatial resolution of the reference image, and ‘SplineOrder’ denotes the number of spline basis functions defined per spatial dimension.
